# Supplementary material for: Systems-level approach to uncovering diffusive states and their transitions from single particle trajectories
Source: arXiv:1608.01419 source file (2016-08-04)
Supplement: Supplementary file 1 [file supp.pdf]

# Supplemental Materials

## Systems-level approach to uncovering diffusive states and their transitions from single particle trajectories

Peter K. Koo[1], Simon G. J. Mochrie[1,2,*]

**1** Department of Physics, Yale University, New Haven, CT, USA

**2** Department of Applied Physics, Yale University, New Haven, CT, USA

Figure S1. Comparison between MSD and MLE analyses on simulated particle trajectories undergoing confined diffusion *without* localization noise. The average diffusivity estimates (top row) and confinement size estimates (bottom row) from MSD analysis (cyan) and MLE analysis (red) applied to synthetic particle tracks with N=30, 60, 120, or 240 steps, undergoing confined diffusion for various confinement sizes, plotted as a function of the reduced confinement size, $L_{reduced} = \sqrt{\frac{L^{sim,2}}{12D^{sim}\Delta t}}$, with $D^{sim} = 0.3\ \mu m^2 s^{-1}$ and $\Delta t = 0.032$ s. The black dashed line represents the ground truth, *i.e.* the simulated values. The number of particle tracks simulated for track lengths, N=30, 60, 120, and 240 steps, was 400, 200, 100, and 50, respectively. Error bars represent the observed standard deviations.

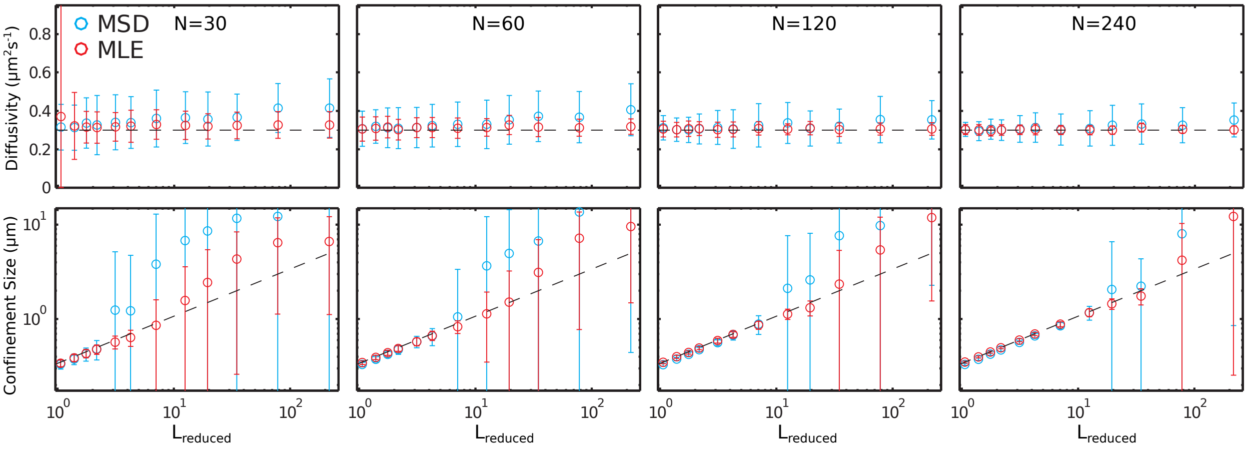

Figure S2. Comparison between MSD and MLE analyses on simulated particle trajectories undergoing fractional Brownian motion *without* localization noise. The average diffusivity estimates (top row) and anomalous exponent estimates (bottom row) from MSD analysis (cyan) and MLE analysis (red) applied to synthetic particle tracks with N=30, 60, 120, or 240 steps, undergoing fractional Brownian motion with various anomalous exponents, plotted as a function of the simulated anomalous exponent, $\alpha^{sim}$, with $D^{sim} = 0.3\ \mu\text{m}^2\text{s}^{-1}$ and $\Delta t = 0.032$ s. The black dashed line represents the ground truth, *i.e.* the simulated values. The number of particle tracks simulated for track lengths, N=30, 60, 120, and 240 steps, was 400, 200, 100, and 50, respectively. Error bars represent the observed standard deviations.

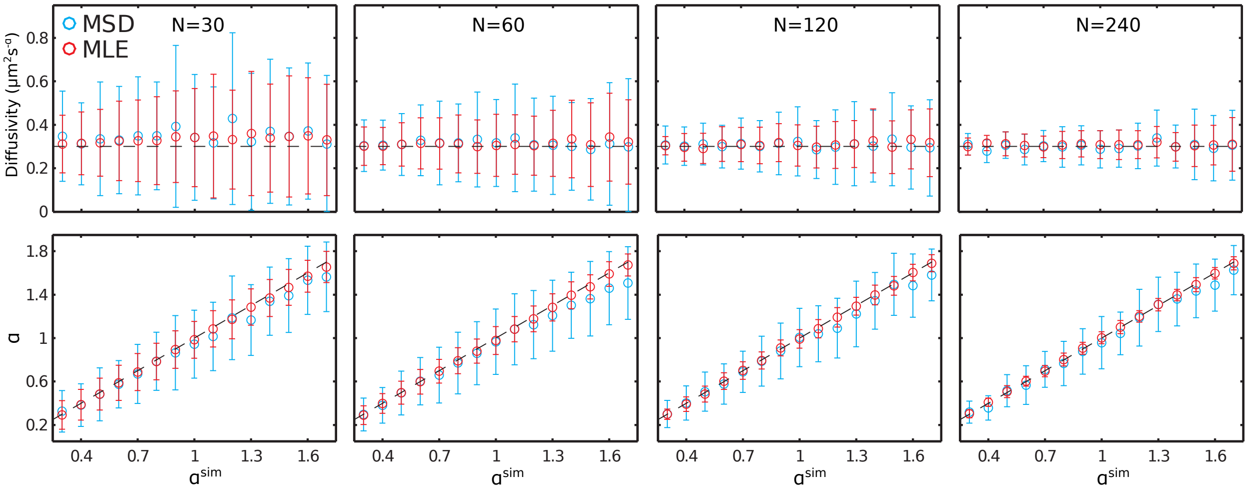

Figure S3. Comparison between MSD and MLE analyses on simulated particle trajectories undergoing confined diffusion *with* localization noise. The average diffusivity estimates (top row) and confinement size estimates (bottom row) from MSD analysis (cyan) and MLE analysis (red) applied to synthetic particle tracks with N=30, 60, 120, or 240 steps, undergoing confined diffusion for various confinement sizes, plotted as a function of the simulated reduced confinement size, $L_{reduced} = \sqrt{\frac{L^{sim,2}}{12D^{sim}\Delta t}}$, with $D^{sim} = 0.3\ \mu\text{m}^2\text{s}^{-1}$, $\Delta t = 0.032$ s, and $\sigma^{sim} = 0.04\ \mu$m. The black dashed line represents the ground truth, *i.e.* the simulated values. The number of particle tracks simulated for track lengths, N=30, 60, 120, and 240 steps, was 400, 200, 100, and 50, respectively. Error bars represent the observed standard deviations. For the MSD analysis, the static localization noise was fixed at the simulated value.

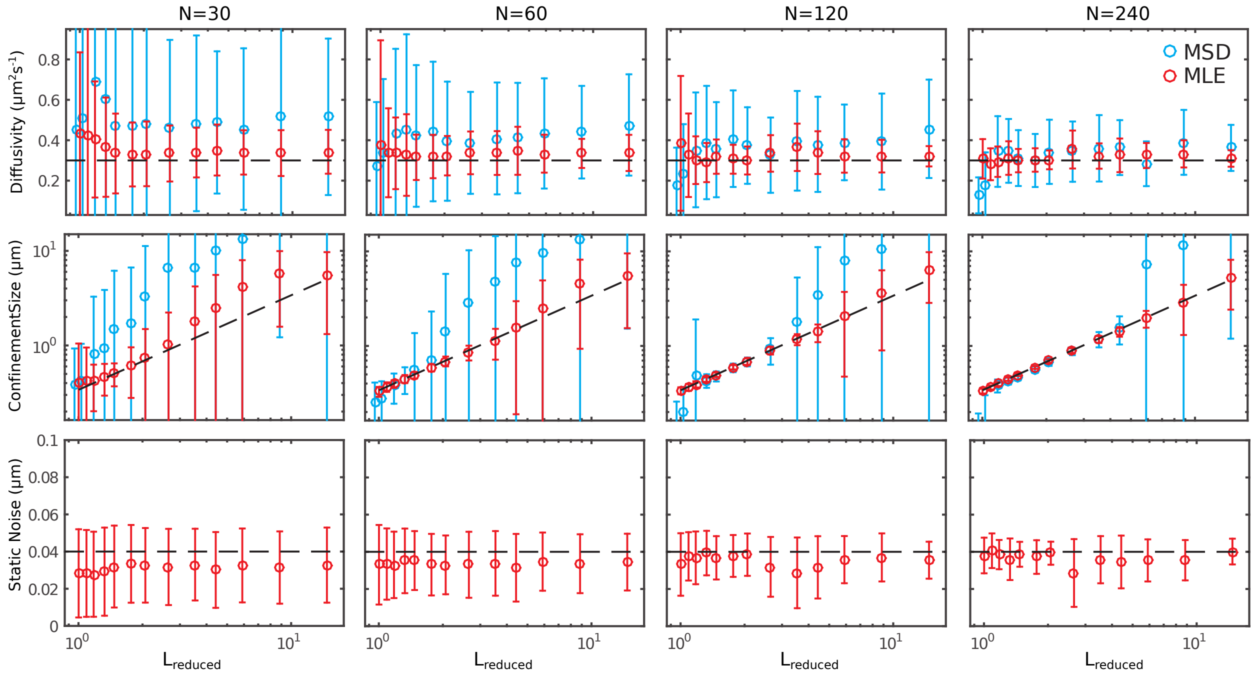

Figure S4. Comparison between MSD and MLE analyses on simulated particle trajectories undergoing fractional Brownian motion *with* localization noise. The average diffusivity estimates (top row) and anomalous exponent estimates (middle row) from MSD analysis (cyan) and MLE analysis (red) applied to synthetic particle tracks with N=30, 60, 120, or 240 steps, undergoing fractional Brownian motion with various anomalous exponents, plotted as a function of the simulated anomalous exponent, $\alpha^{sim}$, with $D^{sim} = 0.3\ \mu\text{m}^2\text{s}^{-1}$, $\Delta t = 0.032$ s, and $\sigma^{sim} = 0.04\ \mu$m. The black dashed line represents the ground truth, *i.e.* the simulated values. The number of particle tracks simulated for track lengths, N=30, 60, 120, and 240 steps, was 400, 200, 100, and 50, respectively. Error bars represent the observed standard deviations. For the MSD analysis, the static localization noise was fixed at the simulated value.

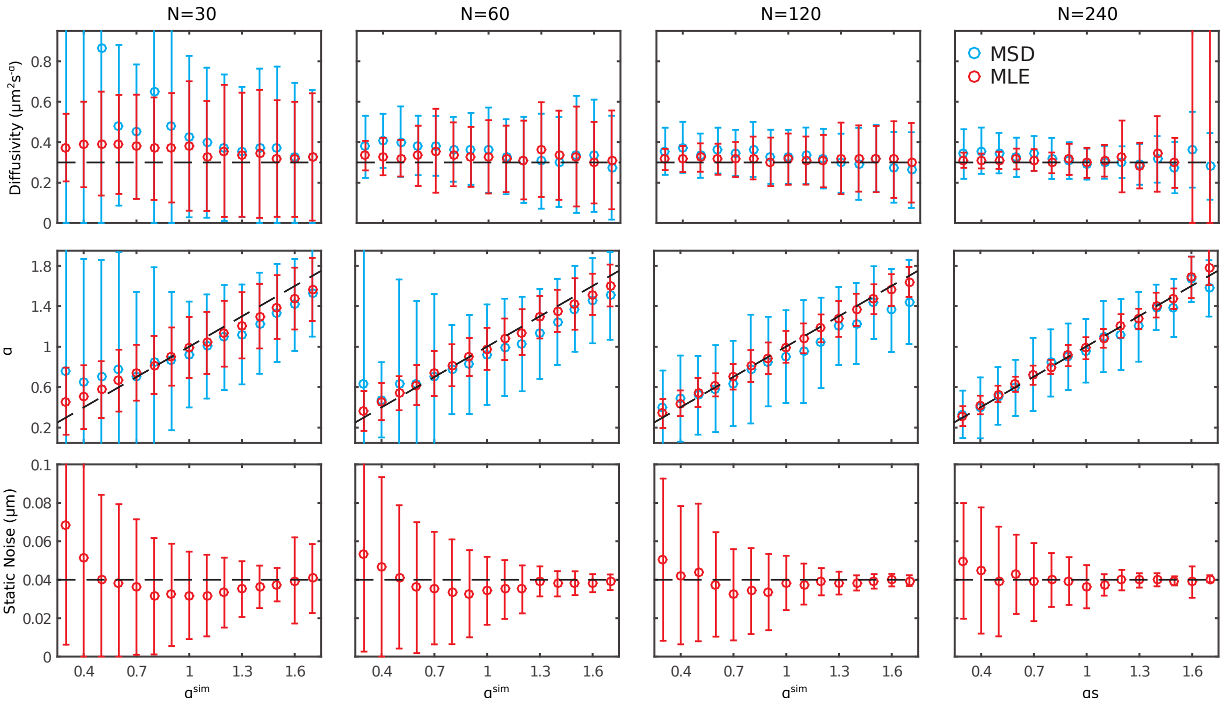

Figure S5. The log-likelihood surface from a representative simulated particle trajectory undergoing confined diffusion. (A) Shows a surface plot and (B) shows a contour plot of the likelihood surface of a representative simulated particle trajectory with $D^{sim} = 0.3\ \mu\text{m}^2\text{s}^{-1}$, $\sigma^{sim} = 0.04\ \mu\text{m}$, $L^{sim} = 0.5\ \mu\text{m}$ for N=30, 60, 120, and 240 steps. The surface is mapped by calculating the likelihood function at equally-spaced confinement sizes and diffusivities. The red marker in each plot represents the maximum likelihood determined by mleBIC's numerical search, while the black marker represents the likelihood value calculated with the simulated parameters, *i.e.* the ground truth. To calculate each likelihood surface, the static localization noise is kept constant at its known value, but takes its optimum value in the mleBIC analysis. Each contour is separated in (B) with 30 equally spaced values, determined by $(\max[\mathcal{L}] - \min[\mathcal{L}])/30$, where $\mathcal{L}$ is the empirical likelihood surface.

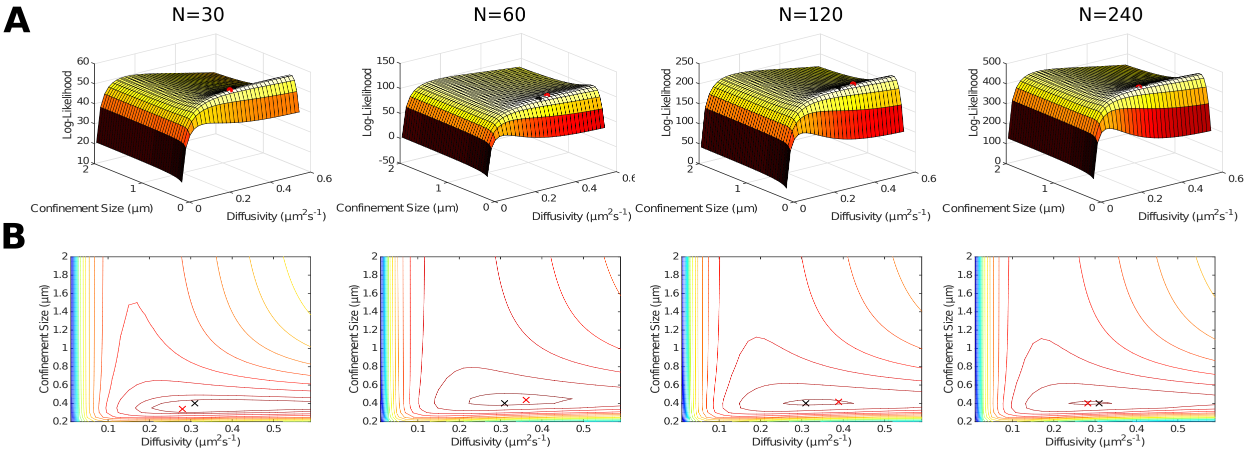

Figure S6. The log-likelihood surface from a representative simulated particle trajectory undergoing fractional Brownian motion. (A) Shows a surface plot and (B) shows a contour plot of the likelihood surface of a representative simulated particle trajectory with $D^{sim} = 0.3\ \mu\text{m}^2\text{s}^{-1}$, $\sigma^{sim} = 0.04\ \mu\text{m}$, $\alpha^{sim} = 0.7$ for N=30, 60, 120, and 240 steps. The surface is mapped by calculating the likelihood function at equally-spaced anomalous exponents and diffusivities. The red marker in each plot represents the maximum likelihood determined by mleBIC's numerical search, while the black marker represents the likelihood value calculated with the simulated parameters, *i.e.* the ground truth. To calculate each likelihood surface, the static localization noise is kept constant at its known value, but takes its optimum value in the mleBIC analysis. Each contour is separated in (B) with 30 equally spaced values, determined by $(\max[\mathcal{L}] - \min[\mathcal{L}])/30$, where $\mathcal{L}$ is the empirical likelihood surface.

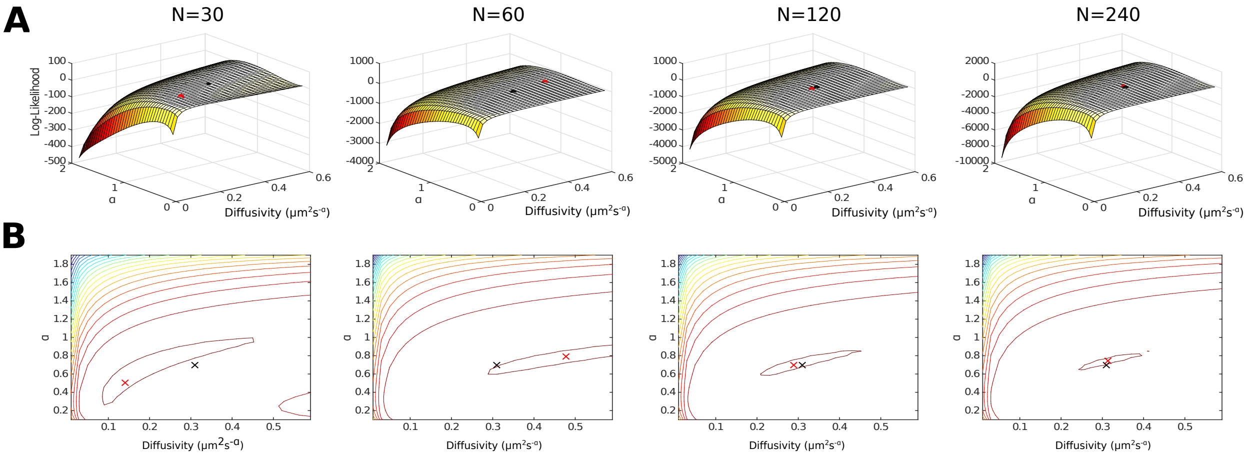

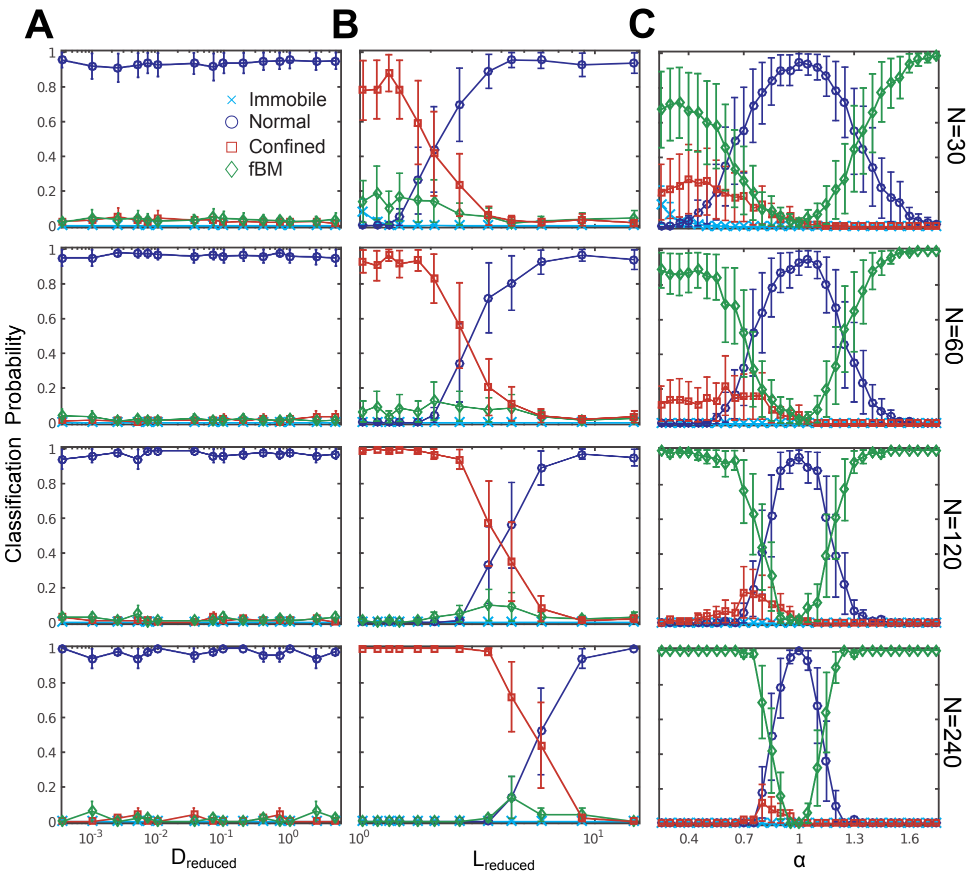


Figure S7. Classification by mleBIC of simulated particle trajectories *without* localization noise for various particle track lengths, undergoing (A) normal diffusion for various underlying diffusivities, (B) confined diffusion for various reduced confinement sizes, and (C) fractional Brownian motion for various anomalous exponents. The probability of each model was calculated on the basis of the fraction of tracks classified to that model at each point in parameter space, and is specified by a unique marker and color: immobile (cyan cross), normal diffusion (blue circles), confined diffusion (red square), and anomalous diffusion (green diamond). Error bars represent the observed standard deviation

Figure S8. Bin size dependence of average transition matrix estimates by pEMv2 classification for synthetic particle tracks, corresponding to case 3. The means of the diagonal elements of the transition matrix, $A_{i,i}$ are plotted as a function of bin size for $i = \{1,\ 2,\ 3\}$ shown in red, green, and blue, respectively. The solid lines linking the data points are guides-to-the-eye. The error bars correspond to the standard deviation of the mean across five trials. The horizontal dashed lines represent the simulated values of the transition matrix elements.

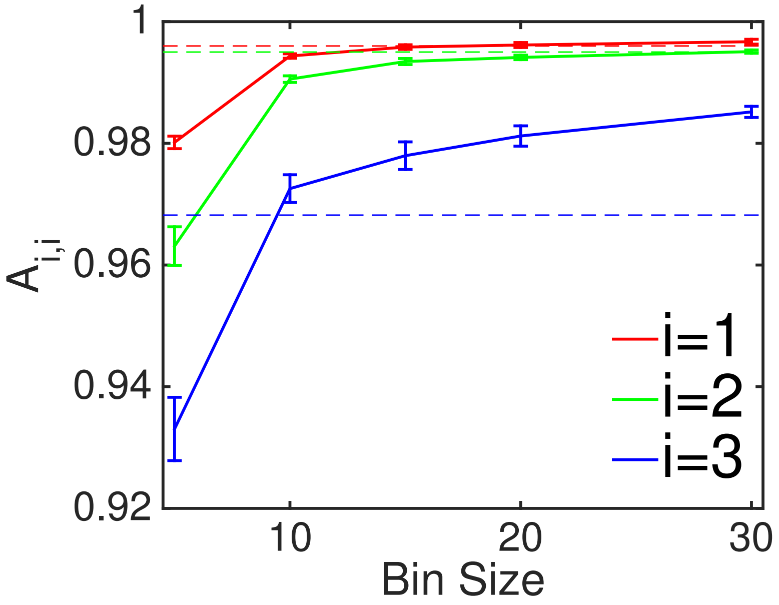

Figure S9. Bin size dependence of pEMv2 classification for a representative particle trajectory with diffusive states given according to case 3. (A) The leftmost panel shows a simulated trajectory that starts off in state 1 (blue), then transitions to state 3 (red), and then transitions to state 2 (green). Subsequent panels show the same trajectory with the color corresponding to the classified state at each point in the trajectory using bin sizes of $B$=5 steps, $B$=10 steps, $B$=20 steps, and $B$=30 steps from left to right. The scale bar represents 200 nm. (B) shows the simulated state sequence (blue line) at each step of the trajectory and the maximum posterior-classified state sequence (red dots) for $B$=5 steps, $B$=15 steps, $B$=20 steps, and $B$=30 steps from left to right.

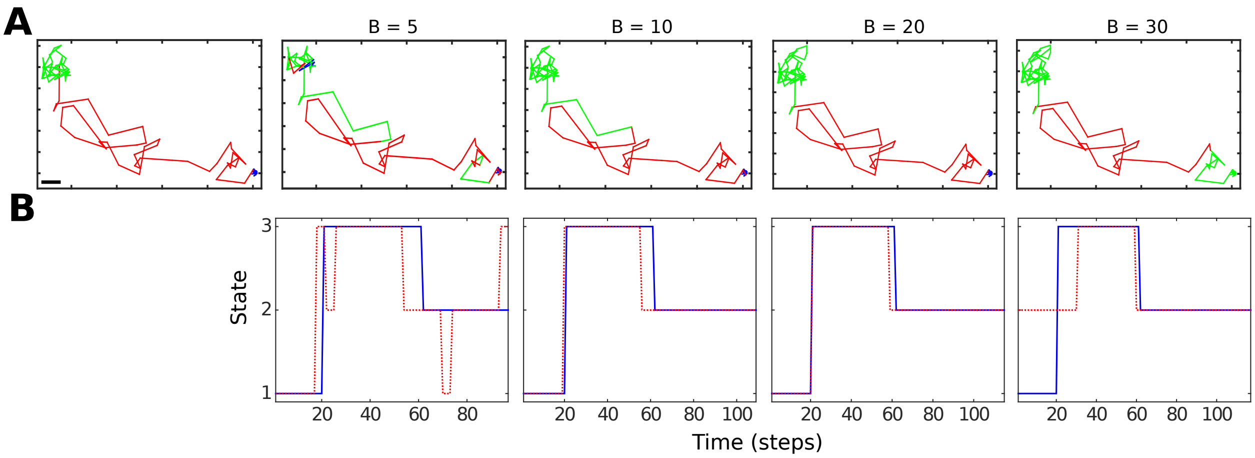

Figure S10. Performance of pEMv2 on binned particle trajectories with diffusive states corresponding to case 4 for several different values of the mean number of transitions per trajectory, $R = \{0,\ 0.6,\ 2.4,\ 3.6\}$. (A) Log-probability versus model size for various bin sizes, each of which is shown in a different color. The results for each number of transitions per trajectory is given in their respective columns (labelled at the top). Each curve represents the log-probability versus model size for five different data sets, each of which is shown as a different curve. The inset shows a zoomed in view of the main figure. (B) Mean fraction of correctly classified diffusive states versus the number of covariance features, namely $N(f+1)$, used in the pEMv2 analysis, where $N$ is the size of the model and $f = 6$ is the number of unique off-diagonal covariance matrix elements. Each data point represents the average of five different sets of simulated particle tracks and the error bars represent their observed standard deviation.

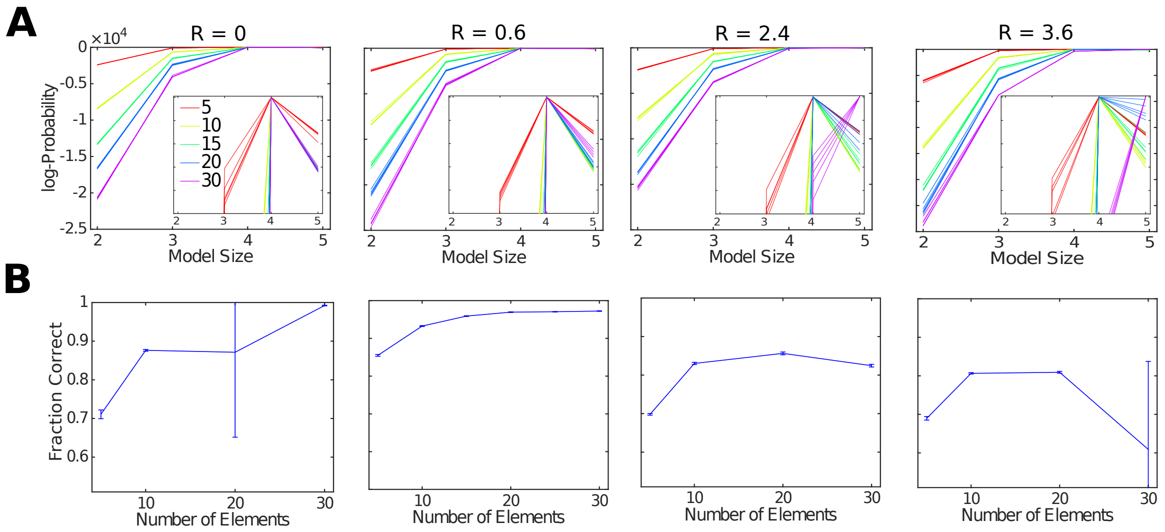

Figure S11. Performation of pEMv2 estimation on particle tracks with diffusive states corresponding to case 4 for several different values of the mean number of transitions per trajectory, $R = \{0,\ 0.6,\ 2.4,\ 3.6\}$. (A) Average covariance matrix elements and (B) average taMSD for each diffusive state determined by maximum posterior classification as a function of time lag for states 1, 2, 3, and 4 represented in red, green, blue and cyan, respectively. (C) Average diagonal elements of the estimated transition matrix, $A_{i,i}$ is plotted as a function of bin size for $i = \{1,\ 2,\ 3,\ 4\}$ shown in red, green, blue, and magenta respectively. In each of (A), (B) and (C), each data point represents the average over five different sets of simulated particle tracks, the solid lines linking the data points are guides-to-the-eye, and the error bars represent the standard deviation of the mean across five trials. In (A) and (B), shown as the dashed curves are the true matrix elements and the true ensemble-averaged taMSD for each state, determined using the known diffusive states of trajectories, while the shaded bands represent its standard deviation. In (C), the horizontal dashed lines represent the simulated values of the transition matrix elements.

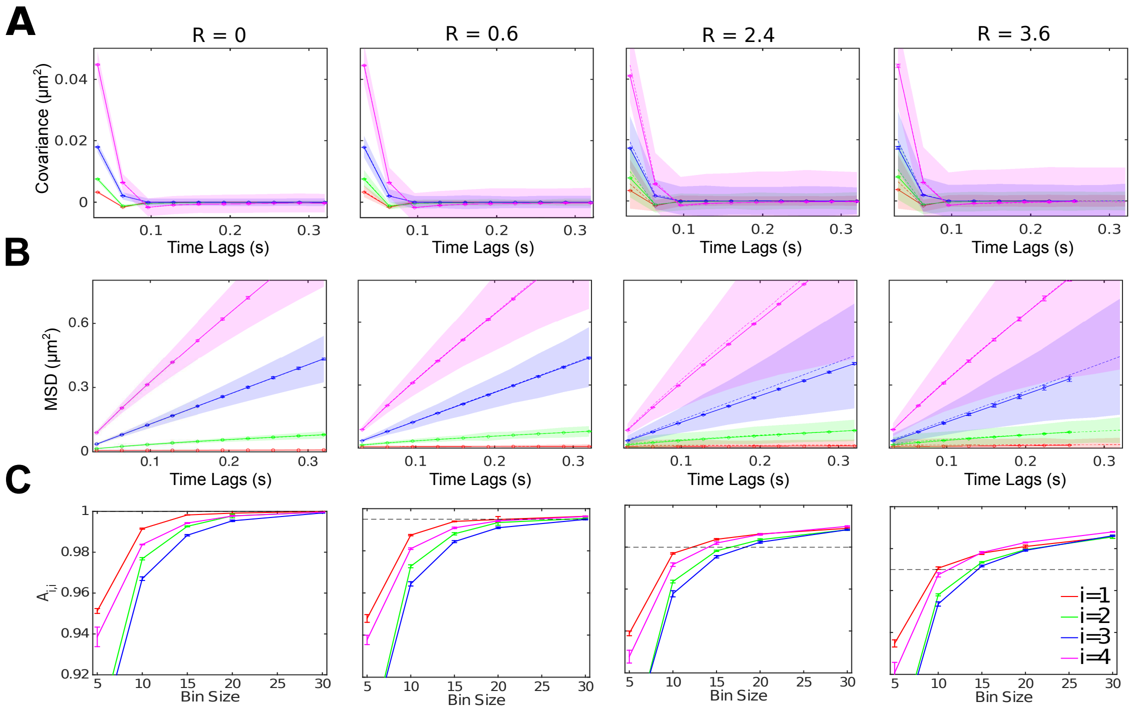

Figure S12. Bin size dependence of pEMv2 classification for a representative particle trajectory with diffusive states corresponding to case 4, with $A = 0.97$. (A) The leftmost panel shows a simulated trajectory that starts off in state 1 (blue), transitions to state 2 (green) after 25 steps, and then transitions back to state 1 (blue) after 72 steps. Subsequent panels from left to right show the same trajectory with the color corresponding to the classifed state at each point in the trajectory for bin sizes of $B$=5 steps, $B$=15 steps, and $B$=30 steps. The portions of the trajectory for $B = 5$, depicted in red, correspond to classification to state 3. The scale bar represents 200 nm. (B) shows the simulated state sequence (blue line) at each step of the trajectory and the maximum posterior-classified state sequence (red dots) for $B$=5 steps, $B$=15 steps, and $B$=30 steps.

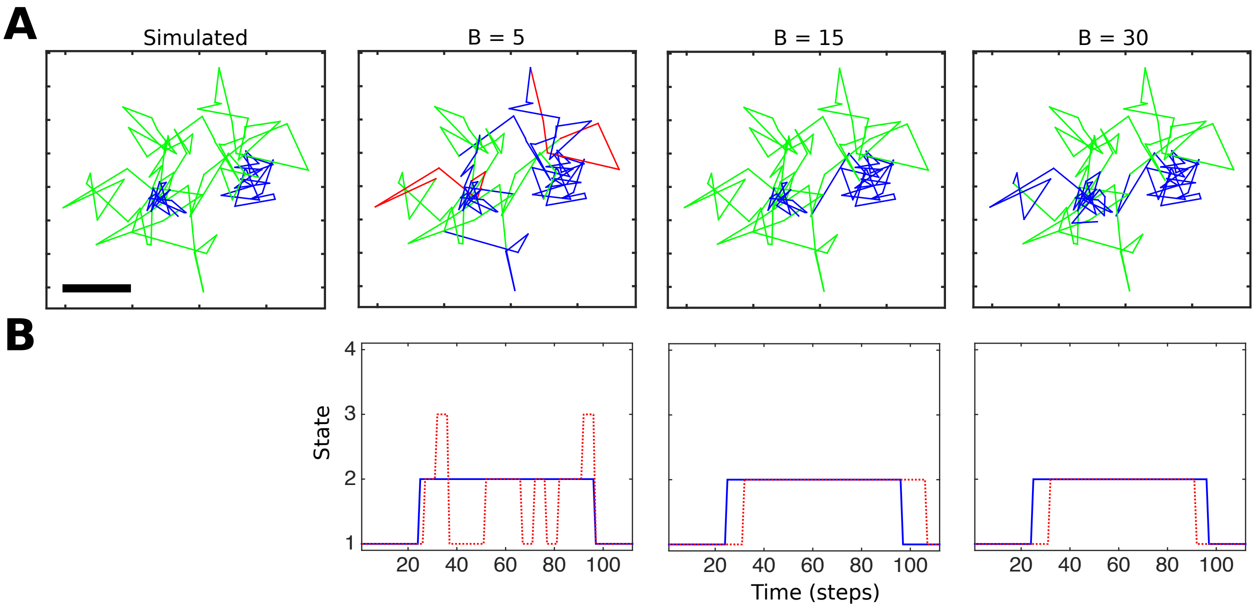

Figure S13. Bin size dependence of pEMv2 classification for a representative particle trajectory with diffusive states corresponding to case 4, with $A = 0.97$. (A) shows a simulated trajectory that starts off in state 1 (blue), then transitions to state 3 (red), then transitions to state 2 (green), then transitions back to state 1 (blue), then transitions back to state 3 (red), and finally back to state 2 (green). Subsequent panels from left to right show the same trajectory with the color corresponding to the classifed state at each point in the trajectory for bin sizes of $B$=5 steps, $B$=15 steps, and $B$=30 steps. The portions of the trajectory for $B = 5$, depicted in cyan, represent classification to state 4. The scale bar represents 200 nm. (B) shows the simulated state sequence (blue line) at each step of the trajectory and the maximum posterior-classified state sequence (red dots) for $B$=5 steps, $B$=15 steps, and $B$=30 steps.

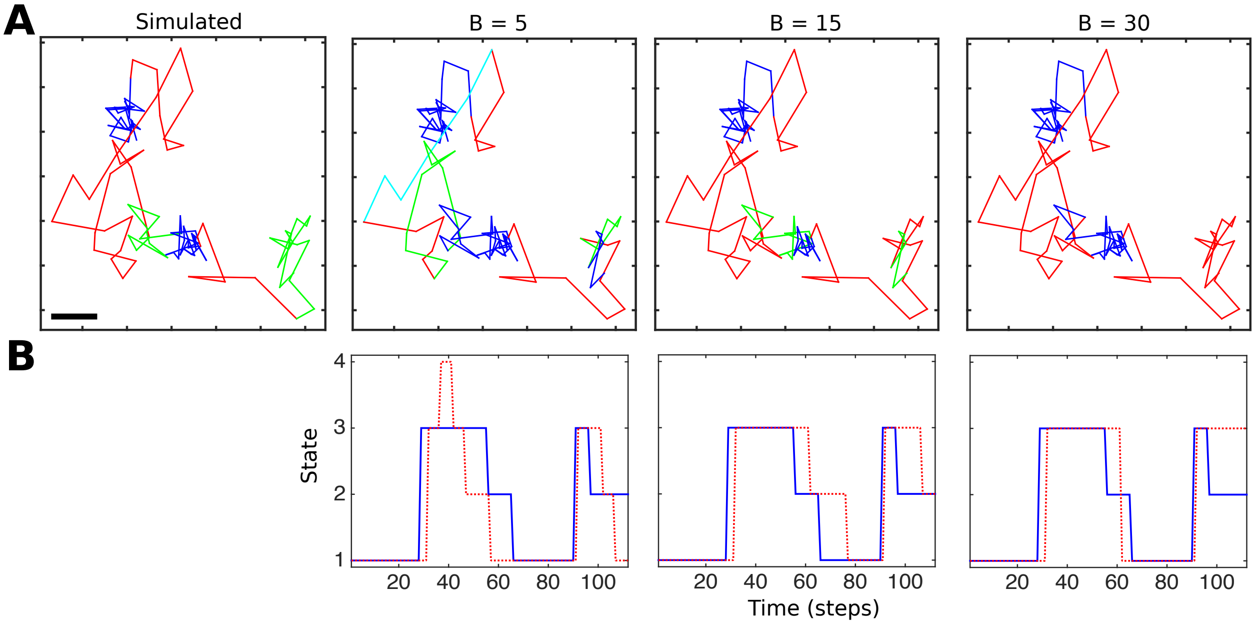

## S1. ISSUES WITH THE TIME-AVERAGED MEAN SQUARE DISPLACEMENT ANALYSIS

Traditionally, analysis of the diffusion properties of single particle tracking data relies on the ensemble-averaged mean square displacement (eaMSD) [1, 2]. For a collection of $M$ 1-dimensional (1D) particle trajectories, where particle trajectory $m$ consists of positions $\mathbf{x}_m = \{x_m(0), x_m(1), ..., x_m(T)\}$, the eaMSD for the $n$th time lag, $\rho_n$, is calculated according to:

$$\rho_n = \frac{1}{M}\sum_{i=1}^{M}\left(x_m(n) - x_m(0)\right)^2 \ .$$

The analytical forms of the eaMSD for several canonical diffusion models, namely normal diffusion, confined diffusion, and anomalous diffusion, are given in Table S5 [2–4]. Figure S23A illustrates the characteristic trends in the eaMSD for each of these models. For normal diffusion (blue curve), the eaMSD increases linearly with time lag. For driven diffusion (orange curve), the eaMSD increases parabolically with time lag [3]. For confined diffusion (red curve), the eaMSD initially increases linearly with time lag and but then plateaus to the value $L^2/6$. For anomalous diffusion, the eaMSD increases with time lag according to a power law, where an anomalous exponent $\alpha < 1$ represents anomalous sub-diffusion (green curve), and $\alpha > 1$ represents anomalous super-diffusion (not shown). By employing the eaMSD, the ensemble diffusive behavior of a collection of single particle trajectories can be quantified by applying a least squares fit for each diffusion model and subsequently assessing the quality of each fit in a statistical manner [2].

Employing the eaMSD, however, makes the assumption that all of the particle trajectories in the average share similar diffusion properties, implying that all of the particles experience

| Mode | 1D eaMSD Model |
|---|---|
| Normal | $2D\Delta t$ |
| Confined | $\frac{L^2}{6} - \frac{16L^2}{\pi^4}\sum_{k=1,odd}^{\infty}\frac{1}{k^4}\exp\left[-\left(\frac{k\pi}{L}\right)^2 D\Delta t\right]$ |
| Anomalous | $2D\Delta t^{\alpha}$ |

Table S1. Ensemble-average MSD model for various modes of diffusion. $D$ is the diffusion coefficient, $L$ is the confinement size, $\alpha$ is the anomalous exponent, and $\Delta t$ is the time between positions.

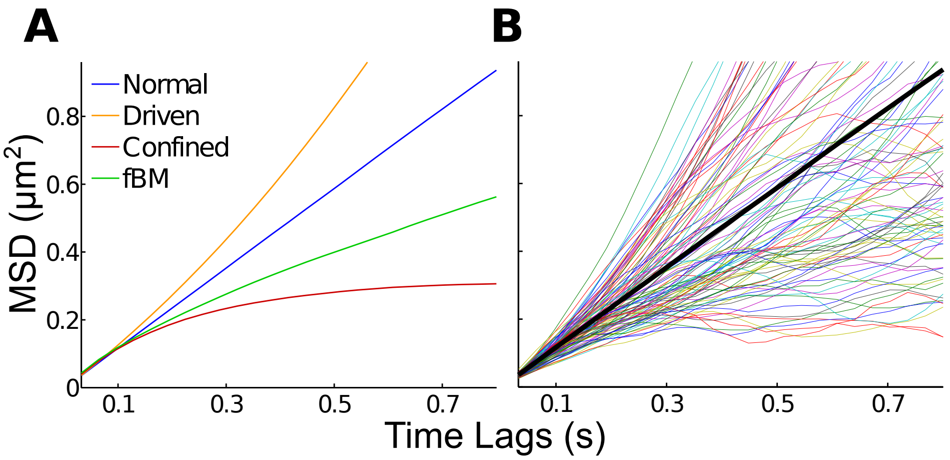


Figure S14. Comparison of eaMSD and taMSD. (Left) The first 25 time lags of the eaMSD calculated from 1,000 simulated particle trajectories each with 50 steps separated in time by $\Delta t = 0.032$ s is shown for normal diffusion (blue), driven diffusion (orange), confined diffusion (red) and anomalous diffusion (green). (Right) 100 representative taMSD curves from the simulated particle trajectories undergoing normal diffusion, with diffusion coefficient $D = 0.3\ \mu\text{m}^2\text{s}^{-1}$.

the same interactions. In live cells, however, diffusing particles can undergo numerous kinds of interactions, either with other particles or with their local environment. Thus, eaMSD analysis inevitably averages over any heterogeneity in diffusive behavior, thereby nullifying the benefits of single molecule investigation.

To preserve heterogeneity across particle trajectories, the time-averaged mean square displacement (taMSD) can be employed in lieu of the eaMSD. For a stationary sequence of $T$ 1D particle positions, $\mathbf{x} = \{x(t)\}$ for $t = 1$ through $T$, each separated one from the next by a time, $\Delta t$, the taMSD is commonly calculated according to [3, 4]:

$$\overline{\delta(\Delta_n, T)} = \frac{1}{T - \Delta_n} \sum_{t=1}^{T-\Delta_n} \left(x(t + \Delta_n) - x(t)\right)^2$$

where $\overline{\delta(\Delta_n, T)}$ is the taMSD for the $n$th time lag, $\Delta_n = n\Delta t$ and the bar on top of $\delta(\Delta_n, T)$ is used to distinguish the time average.

In analyzing individual particle trajectories via time-averages, we make the underlying assumption that the governing motion is ergodic, which means the time-averaged diffusive behavior is representative of its ensemble-averaged diffusive behavior. Thus, the analytical equations which describe the ensemble behavior in Table S5 can also be used to analyze the taMSD. Due to the stochastic nature of diffusion, however, the equivalence only holds in the

limit of infinitely-long particle trajectories [5]. Experimental particle trajectories, however, have finite length. Thus, the ergodicity condition cannot be satisfied.

Moreover, the way in which the taMSD is calculated intrinsically increases the statistical complexity of the taMSD. In particular, the taMSDs across different time lags are serially correlated, because the same information is repeatedly drawn for each time lag. In addition, the samples from within a given time lag can also be correlated when displacements overlap. Furthermore, the taMSD is structured to have one less squared displacement in the average with increasing time lag, contributing to an increasing variance with increasing time lag, a phenomenon known as heteroskedasticity [6].

Due to the statistical complexity of the taMSD, characterizing the long-time diffusive behavior on the basis of the taMSD is challenging. Figure S23B shows 100 taMSD curves calculated from simulated trajectories undergoing normal diffusion, used to generate the eaMSD in Figure S23a. The progressively increasing scatter of the taMSDs for higher time lags results in significant deviations from linear behavior. Consequently, the trends in a significant portion of the taMSD curves appear to show confined, driven, or anomalous diffusion. Hence, the taMSD cannot be trusted for diffusion analysis, especially when using an unweighted least squares fit, as is commonly done, due to the artifacts which arise as a result of limited statistics.

According to the Gauss-Markov theorem [7], ordinary least squares fitting does not provide optimum parameter estimates when the data exhibit heteroskedasticity and serial correlations. Proper statistical treatment of both heteroskedasticity and serial correlations is achieved with Generalized Least Squares (GLS) which seeks to minimize the residuals weighted with the inverse covariance matrix of the taMSD, $\Gamma$, according to [6]:

$$\hat{\beta} = \arg\min_{b} \left[ (\rho - \overline{\delta})^T \Gamma^{-1} (\rho - \overline{\delta}) \right]$$

where $\overline{\delta}$ is the empirical taMSD and $\rho$ is the theoretical mean square displacement solution for a candidate diffusion model. Implementation of GLS, however, requires prior knowledge of $\Gamma$. In practice, this can be obtained either by directly estimating the covariance matrix from the particle trajectories themselves [8] or by utilizing an analytical form [9]. Direct estimation has the benefit of a diffusion model free approach with applications beyond normal diffusion; however, the construction of an accurate empirical covariance matrix requires either a very long particle trajectory, or by calculating the covariance of the taMSD curves across multiple

particle trajectories which must therefore have similar underlying diffusion properties [8]. When there exists heterogeneity across particle trajectories, selection of which trajectories share the same underlying diffusion properties, to average in the construction of the empirical covariance matrix, is not at all straightforward.

On the other hand, the analytical form of the covariance matrix for normal diffusion depends on the parameters under investigation, namely the diffusion coefficient ($D$) and static localization noise ($\sigma$) [3, 10]. Hence, an iterative scheme, known as feasible GLS (fGLS) [6], can be employed to generate the analytical covariance matrix directly from an individual particle trajectory. First, the covariance matrix is constructed with a guess of the parameters, and then GLS is employed to generate a better estimate of the parameters. This process is then iterated until the values of $D$ and $\sigma$ converge. Although the theoretical performance of GLS is at the Cramer-Rao lower bound (CRLB), which is the information theoretic limit for the errors of an estimate, the iterative version fGLS has been found to be slightly biased for normal diffusion [9]. Since the analytical form of the covariance matrix has been available solely for normal diffusion until recently, the extension of fGLS to other diffusion modes remains untested.

## S2. DERIVATION OF THE COVARIANCE MATRIX FOR A PARTICLE UNDERGOING NORMAL DIFFUSION CONFINED IN A FINITE GEOMETRY

For a particle undergoing normal diffusion with a diffusion coefficient, $D$, confined in a finite square geometry of size, $L$, with reflecting boundary conditions, the probability that the particle starts at position $x_0$ at time $t_0$ and is located at position $x$ at time $t$ is given by the propagator [11]:

$$P(x,t|x_0,t_0) = \frac{1}{L} + \frac{2}{L}\sum_{k=1}^{\infty}\cos\left(\frac{k\pi x}{L}\right)\cos\left(\frac{k\pi x_0}{L}\right)\exp\left[-\left(\frac{k\pi}{L}\right)^2 D(t-t_0)\right].$$

The covariance matrix can be constructed by directly calculating:

$$\mathbf{\Sigma}(i,j) = \langle (x_{i+1}-x_i)(x_{j+1}-x_j)\rangle\,.$$

To simplify this calculation, we separate the covariance matrix into 3 different regimes: 1. diagonal elements, 2. nearest-neighbor covariance, and 3. higher order covariance terms.

### 1. Diagonal elements

Given the fact that a particle trajectory can begin at a random location in the domain $[0, L]$, and the initial positions, $x_0$, are equally probable, the initial distribution at time $t_0$ is given by a uniform distribution, $P(x_0, t_0) = \frac{1}{L}$. The equilibrium diagonal elements of the covariance matrix of the particle track displacements averaged over all initial positions can be calculated according to:

$$\begin{aligned}
\left\langle (x-x_0)^2\right\rangle_{eq} &= \int_0^L dx \int_0^L dx_0\ (x-x_0)^2 P(x,x_0,t,t_0)\\
&= \int_0^L dx \int_0^L dx_0\ (x-x_0)^2 P(x,t|x_0,t_0)P(x_0,t_0)\\
&= \int_0^L dx \int_0^L dx_0\ (x^2+x_0^2-2xx_0)\\
&\quad\times\left(\frac{1}{L}+\frac{2}{L}\sum_{k=1}^{\infty}\cos\left(\frac{k\pi x}{L}\right)\cos\left(\frac{k\pi x_0}{L}\right)\exp\left[-\left(\frac{k\pi}{L}\right)^2 D\Delta t\right]\right)\frac{1}{L}\\
&= \frac{1}{L^2}\int_0^L dx\int_0^L dx_0\ x^2+x_0^2-2xx_0\\
&\quad+\frac{2}{L^2}\sum_{k=1}^{\infty}\int_0^L dx\int_0^L dx_0\ (x^2+x_0^2-2xx_0)\cos\left(\frac{k\pi x}{L}\right)\cos\left(\frac{k\pi x_0}{L}\right)\exp\left[-\left(\frac{k\pi}{L}\right)^2 D\Delta t\right]\\
&= \frac{L^2}{6}+\frac{2}{L^2}\sum_{k=1}^{\infty}\frac{-8L^4}{k^4\pi^4}\left(\cos^2[k\pi]+1-2\cos[k\pi]\right)\exp\left[-\left(\frac{k\pi}{L}\right)^2 D\Delta t\right]\\
&= \frac{L^2}{6}-\frac{16L^2}{\pi^4}\sum_{k=1,odd}^{\infty}\frac{1}{k^4}\exp\left[-\left(\frac{k\pi}{L}\right)^2 D\Delta t\right],
\end{aligned}$$

which is the standard mean square displacement solution for confined diffusion [11].

2. Nearest-neighbor covariance

Similarly, the equilibrium nearest-neighbor covariance is given according to

$$
\begin{aligned}
\langle (x_2 - x_1)(x_1 - x_0) \rangle_{eq} &= \int_0^L dx_2 \int_0^L dx_1 \int_0^L dx_0 \ (x_2 - x_1)(x_1 - x_0) P(x_2, x_1, x_0, t_2, t_1, t_0) \\
&= \int_0^L dx_2 \int_0^L dx_1 \int_0^L dx_0 \ (x_2 - x_1)(x_1 - x_0) P(x_2, t_2 | x_1, t_1) P(x_1, t_1 | x_0, t_0) P(x_0, t_0) \\
&= \int_0^L dx_2 \int_0^L dx_1 \int_0^L dx_0 \ (x_2 x_1 - x_2 x_0 - x_1^2 + x_1 x_0) \\
&\times \left( \frac{1}{L} + \frac{2}{L} \sum_{k=1}^{\infty} \cos\left(\frac{k\pi x_2}{L}\right) \cos\left(\frac{k\pi x_1}{L}\right) \exp\left[ -\left(\frac{k\pi}{L}\right)^2 D\Delta t \right] \right) \\
&\times \left( \frac{1}{L} + \frac{2}{L} \sum_{k'=1}^{\infty} \cos\left(\frac{k'\pi x_1}{L}\right) \cos\left(\frac{k'\pi x_0}{L}\right) \exp\left[ -\left(\frac{k'\pi}{L}\right)^2 D\Delta t \right] \right) \left(\frac{1}{L}\right) \\
&= \frac{1}{L} \int_0^L dx_2 \int_0^L dx_1 \int_0^L dx_0 \ (x_2 x_1 - x_2 x_0 - x_1^2 + x_1 x_0) \\
&\times \left( \frac{1}{L^2} + \frac{2}{L^2} \sum_{k=1}^{\infty} \cos\left(\frac{k\pi x_2}{L}\right) \cos\left(\frac{k\pi x_1}{L}\right) \exp\left[ -\left(\frac{k\pi}{L}\right)^2 D\Delta t \right] \right. \\
&+ \frac{2}{L^2} \sum_{k'=1}^{\infty} \cos\left(\frac{k'\pi x_1}{L}\right) \cos\left(\frac{k'\pi x_0}{L}\right) \exp\left[ -\left(\frac{k'\pi}{L}\right)^2 D\Delta t \right] \\
&\left. + \frac{4}{L^2} \sum_{k=1}^{\infty} \sum_{k'=1}^{\infty} \cos\left(\frac{k\pi x_2}{L}\right) \cos\left(\frac{k\pi x_1}{L}\right) \cos\left(\frac{k'\pi x_1}{L}\right) \cos\left(\frac{k'\pi x_0}{L}\right) \exp\left[ -\left(\frac{k'\pi}{L}\right)^2 D\Delta t \right] \exp\left[ -\left(\frac{k\pi}{L}\right)^2 D\Delta t \right] \right).
\end{aligned}
$$

Using the symmetry of the integral to eliminate odd and even components and using the orthogonality relationship $\int_0^L \cos\left(\frac{k\pi x}{L}\right) \cos\left(\frac{k'\pi x}{L}\right) dx = \delta_{k,k'} \frac{L}{2}$, this expression simplifies to:

$$
\begin{aligned}
\langle (x_2 - x_1)(x_1 - x_0) \rangle_{eq} &= \frac{1}{L^3} \int_0^L dx_2 \int_0^L dx_1 \int_0^L dx_0 \ (x_2 x_1 - x_2 x_0 - x_1^2 + x_1 x_0) \\
&+ \frac{2}{L^2} \sum_{k=1}^{\infty} \int_0^L dx_2 \int_0^L dx_1 \left( x_2 x_1 \cos\left(\frac{k\pi x_2}{L}\right) \cos\left(\frac{k\pi x_1}{L}\right) \exp\left[ -\left(\frac{k\pi}{L}\right)^2 D\Delta t \right] \right) \\
&+ \frac{2}{L^2} \sum_{k'=1}^{\infty} \int_0^L dx_1 \int_0^L dx_0 \left( x_1 x_0 \cos\left(\frac{k'\pi x_1}{L}\right) \cos\left(\frac{k'\pi x_0}{L}\right) \exp\left[ -\left(\frac{k'\pi}{L}\right)^2 D\Delta t \right] \right) \\
&+ \frac{4}{L^2} \sum_{k=1}^{\infty} \sum_{k'=1}^{\infty} \int_0^L dx_2 \int_0^L dx_1 \int_0^L dx_0 \left( x_2 x_0 \cos\left(\frac{k\pi x_2}{L}\right) \cos\left(\frac{k\pi x_1}{L}\right) \right. \\
&\left. \cos\left(\frac{k'\pi x_1}{L}\right) \cos\left(\frac{k'\pi x_0}{L}\right) \left( \exp\left[ -\left(\frac{k'\pi}{L}\right)^2 D\Delta t \right] \exp\left[ -\left(\frac{k\pi}{L}\right)^2 D\Delta t \right] \right) \right) \\
&= \frac{1}{L} \left( \frac{-L^3}{12} + 2 \frac{8L^3}{\pi^4} \sum_{k=1,odd}^{\infty} \frac{1}{k^4} \exp\left[ -\left(\frac{k\pi}{L}\right)^2 D\Delta t \right] \right) \\
&\left( -\frac{8L^3}{\pi^4} \sum_{k=1,odd}^{\infty} \frac{1}{k^4} \exp\left[ -2\left(\frac{k\pi}{L}\right)^2 D\Delta t \right] \right) \\
&= \frac{-L^2}{12} + \frac{8L^2}{\pi^4} \sum_{k=1,odd}^{\infty} \frac{1}{k^4} \exp\left[ -\left(\frac{k\pi}{L}\right)^2 D\Delta t \right] \left( 2 - \exp\left[ -2\left(\frac{k\pi}{L}\right)^2 D\Delta t \right] \right).
\end{aligned}
$$

3. higher order covariance terms

$$
\begin{aligned}
\langle (x_{n+1}-x_n)(x_1-x_0)\rangle_{eq} &= \int_0^L dx_{n+1}\int_0^L dx_n \int_0^L dx_1 \int_0^L dx_0\ (x_{n+1}-x_n)(x_1-x_0) \\
&\quad \times P(x_{n+1},x_n,x_1,x_0,t_{n+1},t_n,t_1,t_0) \\
&= \int_0^L dx_{n+1}\int_0^L dx_n \int_0^L dx_1 \int_0^L dx_0\ (x_{n+1}-x_n)(x_1-x_0) \\
&\quad \times P(x_{n+1},t_{n+1}|x_n,t_n)P(x_n,t_n|x_1,t_1)P(x_1,t_1|x_0,t_0)P(x_0,t_0) \\
&= \int_0^L dx_{n+1}\int_0^L dx_n \int_0^L dx_1 \int_0^L dx_0\ (x_{n+1}x_1 - x_{n+1}x_0 - x_n x_1 + x_n x_0) \\
&\quad \times \left(\frac{1}{L}+\frac{2}{L}\sum_{k=1}^{\infty}\cos\left(\frac{k\pi x_{n+1}}{L}\right)\cos\left(\frac{k\pi x_n}{L}\right)\exp\left[-\left(\frac{k\pi}{L}\right)^2 D\Delta t\right]\right) \\
&\quad \times \left(\frac{1}{L}+\frac{2}{L}\sum_{k'=1}^{\infty}\cos\left(\frac{k'\pi x_n}{L}\right)\cos\left(\frac{k'\pi x_1}{L}\right)\exp\left[-\left(\frac{k'\pi}{L}\right)^2 D(n-1)\Delta t\right]\right) \\
&\quad \times \left(\frac{1}{L}+\frac{2}{L}\sum_{k''=1}^{\infty}\cos\left(\frac{k''\pi x_1}{L}\right)\cos\left(\frac{k''\pi x_0}{L}\right)\exp\left[-\left(\frac{k''\pi}{L}\right)^2 D\Delta t\right]\right)\left(\frac{1}{L}\right) \\
&= \int_0^L dx_{n+1}\int_0^L dx_n \int_0^L dx_1 \int_0^L dx_0\ (x_{n+1}x_1 - x_{n+1}x_0 - x_n x_1 + x_n x_0) \\
&\quad \times \Bigg\{\frac{1}{L^4}+\frac{2}{L^4}\sum_{k=1}^{\infty}\cos\left(\frac{k\pi x_{n+1}}{L}\right)\cos\left(\frac{k\pi x_n}{L}\right)\exp\left[-\left(\frac{k\pi}{L}\right)^2 D\Delta t\right] \\
&\quad +\frac{2}{L^4}\sum_{k'=1}^{\infty}\cos\left(\frac{k'\pi x_n}{L}\right)\cos\left(\frac{k'\pi x_1}{L}\right)\exp\left[-\left(\frac{k'\pi}{L}\right)^2 D(n-1)\Delta t\right] \\
&\quad +\frac{2}{L^4}\sum_{k''=1}^{\infty}\cos\left(\frac{k''\pi x_1}{L}\right)\cos\left(\frac{k''\pi x_0}{L}\right)\exp\left[-\left(\frac{k''\pi}{L}\right)^2 D\Delta t\right] \\
&\quad +\frac{4}{L^4}\sum_{k=1}^{\infty}\sum_{k'=1}^{\infty}\cos\left(\frac{k\pi x_{n+1}}{L}\right)\cos\left(\frac{k\pi x_n}{L}\right)\cos\left(\frac{k'\pi x_n}{L}\right)\cos\left(\frac{k'\pi x_1}{L}\right) \\
&\quad \times\exp\left[-\left(\frac{k\pi}{L}\right)^2 D\Delta t\right]\exp\left[-\left(\frac{k'\pi}{L}\right)^2 (n-1)D\Delta t\right] \\
&\quad +\frac{4}{L^4}\sum_{k=1}^{\infty}\sum_{k''=1}^{\infty}\cos\left(\frac{k\pi x_{n+1}}{L}\right)\cos\left(\frac{k\pi x_n}{L}\right)\cos\left(\frac{k''\pi x_1}{L}\right)\cos\left(\frac{k''\pi x_0}{L}\right) \\
&\quad \times\exp\left[-\left(\frac{k\pi}{L}\right)^2 D\Delta t\right]\exp\left[-\left(\frac{k''\pi}{L}\right)^2 D\Delta t\right] \\
&\quad +\frac{4}{L^4}\sum_{k'=1}^{\infty}\sum_{k''=1}^{\infty}\cos\left(\frac{k'\pi x_n}{L}\right)\cos\left(\frac{k'\pi x_1}{L}\right)\cos\left(\frac{k''\pi x_1}{L}\right)\cos\left(\frac{k''\pi x_0}{L}\right) \\
&\quad \times\exp\left[-\left(\frac{k'\pi}{L}\right)^2 D(n-1)\Delta t\right]\exp\left[-\left(\frac{k''\pi}{L}\right)^2 D\Delta t\right] \\
&\quad +\frac{4}{L^4}\sum_{k=1}^{\infty}\sum_{k'=1}^{\infty}\sum_{k''=1}^{\infty}\cos\left(\frac{k\pi x_{n+1}}{L}\right)\cos\left(\frac{k\pi x_n}{L}\right) \\
&\quad \times\cos\left(\frac{k'\pi x_n}{L}\right)\cos\left(\frac{k'\pi x_1}{L}\right)\cos\left(\frac{k''\pi x_1}{L}\right)\cos\left(\frac{k''\pi x_0}{L}\right) \\
&\quad \times\exp\left[-\left(\frac{k\pi}{L}\right)^2 D\Delta t\right]\exp\left[-\left(\frac{k'\pi}{L}\right)^2 D(n-1)\Delta t\right]\exp\left[-\left(\frac{k''\pi}{L}\right)^2 D\Delta t\right]\Bigg\}.
\end{aligned}
$$

Similar to step 2, the symmetry of the integral and the orthogonality relations can be

used to simplify the expression to yield:

$$\begin{aligned}
\langle (x_{n+1}-x_n)(x_1-x_0)\rangle_{eq} &= \frac{1}{L^4}\int_0^L dx_{n+1}\int_0^L dx_n\int_0^L dx_1\int_0^L dx_0\ (x_{n+1}x_1 - x_{n+1}x_0 - x_nx_1 + x_nx_0) \\
&+\frac{2}{L^2}\sum_{k'=1}^{\infty}\int_0^L dx_n\int_0^L dx_1\ x_nx_1\cos\left(\frac{k'\pi x_n}{L}\right)\cos\left(\frac{k'\pi x_1}{L}\right) \\
&\times\exp\left[-\left(\frac{k'\pi}{L}\right)^2 D(n-1)\Delta t\right] \\
&+\frac{4}{L^3}\sum_{k=1}^{\infty}\sum_{k'=1}^{\infty}\int_0^L dx_{n+1}\int_0^L dx_n\int_0^L dx_1\ x_{n+1}x_1 \\
&\times\cos\left(\frac{k\pi x_{n+1}}{L}\right)\cos\left(\frac{k\pi x_n}{L}\right)\cos\left(\frac{k'\pi x_n}{L}\right)\cos\left(\frac{k'\pi x_1}{L}\right) \\
&\times\exp\left[-\left(\frac{k\pi}{L}\right)^2 D\Delta t\right]\exp\left[-\left(\frac{k'\pi}{L}\right)^2 (n-1)D\Delta t\right] \\
&+\frac{4}{L^3}\sum_{k'=1}^{\infty}\sum_{k''=1}^{\infty}\int_0^L dx_n\int_0^L dx_1\int_0^L dx_0\ x_nx_0 \\
&\times\cos\left(\frac{k'\pi x_n}{L}\right)\cos\left(\frac{k'\pi x_1}{L}\right)\cos\left(\frac{k''\pi x_1}{L}\right)\cos\left(\frac{k''\pi x_0}{L}\right) \\
&\times\exp\left[-\left(\frac{k'\pi}{L}\right)^2 D(n-1)\Delta t\right]\exp\left[-\left(\frac{k''\pi}{L}\right)^2 D\Delta t\right] \\
&+\frac{4}{L^4}\sum_{k=1}^{\infty}\sum_{k'=1}^{\infty}\sum_{k''=1}^{\infty}\int_0^L dx_{n+1}\int_0^L dx_n\int_0^L dx_1\int_0^L dx_0\ x_{n+1}x_0 \\
&\times\cos\left(\frac{k\pi x_{n+1}}{L}\right)\cos\left(\frac{k\pi x_n}{L}\right)\cos\left(\frac{k'\pi x_n}{L}\right)\cos\left(\frac{k'\pi x_1}{L}\right)\cos\left(\frac{k''\pi x_1}{L}\right)\cos\left(\frac{k''\pi x_0}{L}\right) \\
&\times\exp\left[-\left(\frac{k\pi}{L}\right)^2 D\Delta t\right]\exp\left[-\left(\frac{k'\pi}{L}\right)^2 D(n-1)\Delta t\right]\exp\left[-\left(\frac{k''\pi}{L}\right)^2 D\Delta t\right] \\
&= \frac{-8L^2}{\pi^4}\sum_{k=1,odd}^{\infty}\frac{1}{k^4}\exp\left[-\left(\frac{k\pi}{L}\right)^2 D(n-1)\Delta t\right] \\
&-2\left(\frac{8L^2}{\pi^4}\sum_{k=1,odd}^{\infty}\frac{1}{k^4}\exp\left[-\left(\frac{k\pi}{L}\right)^2 D\Delta t\right]\exp\left[-\left(\frac{k\pi}{L}\right)^2 D(n-1)\Delta t\right]\right) \\
&-\frac{8L^2}{\pi^4}\sum_{k=1,odd}^{\infty}\frac{1}{k^4}\exp\left[-2\left(\frac{k\pi}{L}\right)^2 D\Delta t\right]\exp\left[-\left(\frac{k\pi}{L}\right)^2 D(n-1)\Delta t\right] \\
&= \frac{8L^2}{\pi^4}\sum_{k=1,odd}^{\infty}\frac{1}{k^4}\left\{\exp\left[-\left(\frac{k\pi}{L}\right)^2 D(n-1)\Delta t\right] - 2\exp\left[-\left(\frac{k\pi}{L}\right)^2 Dn\Delta t\right]\right. \\
&\left. +\exp\left[-\left(\frac{k\pi}{L}\right)^2 D(n+1)\Delta t\right]\right\}.
\end{aligned}$$

In summary, the covariance matrix of the true instantaneous positions for normal diffusion confined in a square geometry is given by:

$$\hat{\mathbf{\Sigma}}(i,j)^{confined} = \begin{cases} \frac{L^2}{6} - \frac{16L^2}{\pi^4}\sum_{k=1,odd}^{\infty}\frac{1}{k^4}\Phi(1) & ,\ j=i \\ \frac{-L^2}{12} + \frac{8L^2}{\pi^4}\sum_{k=1,odd}^{\infty}\frac{1}{k^4}\Phi(1)\left(2-\Phi(1)\right) & ,\ j=i\pm 1 \\ \frac{8}{\pi^4}\sum_{k=1,odd}^{\infty}\frac{1}{k^4}\left(-2\Phi(j-i+1)+\Phi(j-i)+\Phi(j-i+2)\right) & ,\ \text{otherwise} \end{cases} \quad \text{(Eq. S1)}$$

where $\Phi_n = \exp\left[-\left(\frac{k\pi}{L}\right)^2 Dn\Delta t\right]$.

## S3. COVARIANCE MATRIX FOR FRACTIONAL BROWNIAN MOTION

Fractional Brownian motion is defined by its position-position correlation given according to [12, 13]:

$$\langle Z(t_1)Z(t_2)\rangle = D(t_1^\alpha + t_2^\alpha - |t_1 - t_2|^\alpha)$$

where $Z(t)$ is a random variable for the position at time $t$, $D$ is the effective diffusion coefficient, and $\alpha$ is the anomalous exponent, known also as the Hurst coefficient, $H = 2\alpha$.

The covariance matrix of the displacements, $\xi_t = Z(t+\Delta) - Z(t)$, which is also known as fractional Gaussian noise, is given by:

$$\begin{aligned}
\langle \xi(t)\xi(s)\rangle &= \langle (Z(t+\Delta) - Z(t))(Z(s+\Delta) - Z(s))\rangle \\
&= \langle Z(t+\Delta)Z(s+\Delta) - Z(t)Z(s+\Delta) - Z(t+\Delta)Z(s) + Z(t)Z(s)\rangle \\
&= \langle Z(t+\Delta)Z(s+\Delta)\rangle - \langle Z(t)Z(s+\Delta)\rangle - \langle Z(t+\Delta)Z(s)\rangle + \langle Z(t)Z(s)\rangle \\
&= D\left((t+\Delta)^\alpha + (s+\Delta)^\alpha - |t-s|^\alpha - (t+\Delta)^\alpha - s^\alpha + |t+\Delta-s|^\alpha\right. \\
&\quad \left. -t^\alpha - (s+\Delta)^\alpha + |t-s-\Delta|^\alpha + t^\alpha + s^\alpha - |t-s|^\alpha\right) \\
&= D(|t-s+\Delta|^\alpha + |t-s-\Delta|^\alpha - 2\,|t-s|^\alpha).
\end{aligned}$$

When $s$ is equal to $t$, the standard mean square displacement solution, $D = 2D\Delta t^\alpha$, is recovered.

## S4. LOCALIZATION NOISE CONTRIBUTION TO THE COVARIANCE MATRIX

### S4.1. Static localization noise contribution

Static localization noise is the error associated with determining a fluorophore's position during image analysis, and is a direct consequence of the limited number of photons emitted by a fluorophore during the camera exposure time. In practice, the estimated position of a particle along with its static localization noise can be determined by applying a least squares fit of the two-dimensional diffraction-limited point spread function using a radially symmetric Gaussian profile or via a maximum likelihood estimator [14].

Below, we derive an analytical form for the contribution of static localization noise to the covariance matrix. If the true position of a particle at time $t$ is given by $\hat{x}_t$ and the measurement error is $\epsilon_t$, then the experimental position of the particle, $x_t = \hat{x}_t + \epsilon_t$. If we now make the assumption that the static localization noise is uncorrelated in time and normally distributed with zero mean and standard deviation, $\sigma$, then $\langle \epsilon_i \epsilon_j \rangle = \sigma^2 \delta_{ij}$. It follows that the covariance matrix in the presence of static localization noise is given by:

$$\begin{aligned}
\langle (x_{i+1} - x_i)(x_{j+1} - x_j) \rangle &= \langle (\hat{x}_{i+1} + \epsilon_{i+1} - \hat{x}_i - \epsilon_i)(\hat{x}_{j+1} + \epsilon_{j+1} + -\hat{x}_j - \epsilon_j) \rangle \\
&= \langle (\Delta \hat{x}_i + \epsilon_{i+1} - \epsilon_i)(\Delta \hat{x}_j + \epsilon_{j+1} - \epsilon_j) \rangle \\
&= \langle \Delta \hat{x}_i \Delta \hat{x}_j \rangle + \langle \epsilon_{i+1} \epsilon_{j+1} \rangle - \langle \epsilon_{i+1} \epsilon_j \rangle - \langle \epsilon_i \epsilon_{j+1} \rangle + \langle \epsilon_i \epsilon_j \rangle + \mathcal{O}(\langle \Delta \hat{x} \epsilon \rangle) \\
&= \hat{\mathbf{\Sigma}}(i,j) + 2\sigma^2 \delta_{i,j} - \sigma^2 \delta_{i,j+1} - \sigma^2 \delta_{i+1,j} \ ,
\end{aligned}$$

where we have made the assumption that localization noise is independent of particle position, *i.e.* $\langle \Delta \hat{x} \epsilon \rangle = \langle \Delta \hat{x} \rangle \langle \epsilon \rangle = 0$.

### S4.2. Dynamic localization noise contribution

Assuming that the fluorophore is a constant emitter of photons throughout the camera exposure time, then the measured intensity effectively acts as a box car filter of the true fluorophor positions. This motion blur has been thoroughly explored for normal diffusion [10, 15–17]. In addition, the analytical form for the covariance matrix of fractional Brownian motion with dynamic localization noise has recently been derived [18], and is is included in Table 1 in the Main Text. Here, we analyze the effect of motion blur on confined diffusion,

following a similar approach to that pursued in Ref [10, 17], where each trajectory is represented as a sequence of microsteps, separated by a duration $\delta t$ and the time between frames is $\Delta t = m\delta t$, where $m$ is the number of micro steps per time between frames.

The position, $x_{k+1}$, is given by the cumulative sum of the micro step displacements, $\Delta x^{(k)}$ starting from position $x_k$, according to the recursion:

$$x_{k+1} = x_k + \sum_{j=1}^{m} \Delta x_j^{(k+1)},$$

or equivalently the cumulative sum of all the micro step displacements for the $k$ frames starting from $x_1$, according to

$$x_{k+1} = x_1 + \sum_{i=1}^{k} \sum_{j=1}^{m} \Delta x_j^{(i)}.$$

For the $(k+1)$th frame, the motion blurred position is given by the average positions given by:

$$\begin{aligned}
\bar{x}^{(k+1)} &= x_{k+1} + \sum_{j=1}^{q-1} \frac{q-j}{q} \Delta x_j^{(k+1)} \\
&= x_1 + \sum_{i=1}^{k} \sum_{j=1}^{m} \Delta x_j^{(i)} + \sum_{j=1}^{q-1} \frac{q-j}{q} \Delta x_j^{(k+1)},
\end{aligned}$$

where $q$ is the number of micro steps during an exposure time, $\Delta t_E = q\delta t$. The exposure time, $\Delta t_E$, must be less than or equal to the frame time, $\Delta t$. Therefore, $q \leq m$.

The displacement of the motion blurred positions is then given according to:

$$\begin{aligned}
\bar{x}^{(k+1)} - \bar{x}^{(k)} &= \sum_{i=1}^{k} \sum_{j=1}^{m} \Delta x_j^{(i)} + \sum_{j=1}^{q-1} \frac{q-j}{q} \Delta x_j^{(k+1)} - \sum_{i=1}^{k-1} \sum_{j=1}^{m} \Delta x_j^{(i)} - \sum_{j=1}^{q-1} \frac{q-j}{q} \Delta x_j^{(k)} \\
&= \sum_{j=1}^{m} \Delta x_j^{(k)} + \sum_{j=1}^{q-1} \frac{q-j}{q} \Delta x_j^{(k+1)} - \sum_{j=1}^{q-1} \Delta x_j^{(k)} + \sum_{j=1}^{q-1} \frac{j}{q} \Delta x_j^{(k)} \\
&= \sum_{j=q}^{m} \Delta x_j^{(k)} + \sum_{j=1}^{q-1} \frac{q-j}{q} \Delta x_j^{(k+1)} + \sum_{j=1}^{q-1} \frac{j}{q} \Delta x_j^{(k)}
\end{aligned}$$

The covariance of the motion blurred displacements is given by:

$$
\begin{aligned}
\left\langle (\bar{x}^{(k+1)} - \bar{x}^{(k)})(\bar{x}^{(i+1)} - \bar{x}^{(i)}) \right\rangle &= \Bigg\langle \left( \sum_{j=q}^{m} \Delta x_j^{(k)} + \sum_{j=1}^{q-1} \frac{q-j}{q} \Delta x_j^{(k+1)} + \sum_{j=1}^{q-1} \frac{j}{q} \Delta x_j^{(k)} \right) \\
&\quad \times \left( \sum_{j'=q}^{m} \Delta x_{j'}^{(i)} + \sum_{j'=1}^{q-1} \frac{q-j'}{q} \Delta x_{j'}^{(i+1)} + \sum_{j'=1}^{q-1} \frac{j'}{q} \Delta x_{j'}^{(i)} \right) \Bigg\rangle \\
&= \left\langle \sum_{j'=q}^{m} \sum_{j=q}^{m} \Delta x_j^{(k)} \Delta x_{j'}^{(i)} \right\rangle + \left\langle \sum_{j'=1}^{q-1} \sum_{j=1}^{q-1} \left( \frac{j}{q} \right) \left( \frac{j'}{q} \right) \Delta x_j^{(k)} \Delta x_{j'}^{(i)} \right\rangle \\
&\quad + \left\langle \sum_{j'=1}^{q-1} \sum_{j=1}^{q-1} \left( \frac{q-j}{q} \right) \left( \frac{q-j'}{q} \right) \Delta x_j^{(k+1)} \Delta x_{j'}^{(i+1)} \right\rangle \\
&\quad + \left\langle \sum_{j'=1}^{q-1} \sum_{j=1}^{q-1} \left( \frac{q-j}{q} \right) \left( \frac{j'}{q} \right) \Delta x_j^{(k+1)} \Delta x_{j'}^{(i)} \right\rangle \\
&\quad + \left\langle \sum_{j'=1}^{q-1} \sum_{j=1}^{q-1} \left( \frac{q-j'}{q} \right) \left( \frac{j}{q} \right) \Delta x_j^{(k)} \Delta x_{j'}^{(i+1)} \right\rangle \\
&\quad + \left\langle \sum_{j'=q}^{m} \sum_{j=1}^{q-1} \left( \frac{q-j}{q} \right) \Delta x_j^{(k+1)} \Delta x_{j'}^{(i)} \right\rangle + \left\langle \sum_{j'=q}^{m} \sum_{j=1}^{q-1} \left( \frac{j}{q} \right) \Delta x_j^{(k)} \Delta x_{j'}^{(i)} \right\rangle \\
&\quad + \left\langle \sum_{j'=1}^{q-1} \sum_{j=q}^{m} \left( \frac{q-j'}{q} \right) \Delta x_j^{(k)} \Delta x_{j'}^{(i+1)} \right\rangle + \left\langle \sum_{j'=1}^{q-1} \sum_{j=q}^{m} \left( \frac{j'}{q} \right) \Delta x_j^{(k)} \Delta x_{j'}^{(i)} \right\rangle
\end{aligned}
$$

To simplify, we now assume that the dominant contribution to the covariance matrix occurs $j' = j$ and that other terms can be neglected. Thus, we find:

$$
\begin{aligned}
\left\langle (\bar{x}^{(k+1)} - \bar{x}^{(k)})(\bar{x}^{(i+1)} - \bar{x}^{(i)}) \right\rangle &= \left( \sum_{j=q}^{m} + \sum_{j=1}^{q-1} \left( \frac{j}{q} \right)^2 + \sum_{j=1}^{q-1} \left( \frac{q-j}{q} \right)^2 \right) \left\langle \Delta x_j^{(k)} \Delta x_j^{(i)} \right\rangle \\
&\quad + \sum_{j=1}^{q-1} \left( \frac{q-j}{q} \right) \left( \frac{j}{q} \right) \left( \left\langle \Delta x_j^{(k+1)} \Delta x_j^{(i)} \right\rangle + \left\langle \Delta x_j^{(k)} \Delta x_j^{(i+1)} \right\rangle \right) \\
&= \left( m - \frac{q}{3} + \frac{1}{3q} \right) \mathbf{\Sigma}_{k,i}(\delta t) + \left( \frac{q}{6} - \frac{1}{6q} \right) \left( \mathbf{\Sigma}_{k+1,i}(\delta t) + \mathbf{\Sigma}_{k,i+1}(\delta t) \right) \\
&= m \mathbf{\Sigma}_{k,i}(\delta t) - \frac{q}{3} \mathbf{\Sigma}_{k,i}(\delta t) + \frac{q}{3} \left( \mathbf{\Sigma}_{k+1,i}(\delta t) + \mathbf{\Sigma}_{k,i+1}(\delta t) \right) + \mathcal{O}\left( \frac{1}{q} \right) \\
&\approx \mathbf{\Sigma}_{k,i}(m\delta t) - \frac{q\delta t}{3m\delta t} \mathbf{\Sigma}_{k,i}(m\delta t) + \frac{q\delta t}{6m\delta t} \left( \mathbf{\Sigma}_{k+1,i}(m\delta t) + \mathbf{\Sigma}_{k,i+1}(m\delta t) \right) \\
&= \mathbf{\Sigma}_{k,i} - \frac{1}{6} \frac{\Delta t_E}{\Delta t} \left( 2\mathbf{\Sigma}_{k,i} - \mathbf{\Sigma}_{k+1,i} - \mathbf{\Sigma}_{k,i+1} \right) \\
&= \mathbf{\Sigma}_{k,i} - R \left( 2\mathbf{\Sigma}_{k,i} - \mathbf{\Sigma}_{k+1,i} - \mathbf{\Sigma}_{k,i+1} \right)
\end{aligned}
$$

where we have defined the motion blur coefficient as $R = \frac{1}{6}\frac{\Delta t_E}{\Delta t}$ [16]. For normal diffusion, this reproduces the known covariance matrix elements in the presence of localization noise.

To test the theoretical covariance matrices, we simulated particle trajectories undergoing confined diffusion for various confinement sizes and particle trajectories undergoing fractional Brownian motion for various anomalous exponents, while keeping the underlying effective diffusion coefficient, static localization noise, and track length fixed at $D^{sim} = 0.3\ \mu\text{m}^2\text{s}^{-\alpha}$, $\sigma^{sim} = 0.04\ \mu\text{m}$, and $N = 100$, respectively. The first five average empirical covariance terms (each shown in a different color) are plotted in Figure S24. Evidently, the analytical covariance matrix elements with localization noise corrections (solid lines) capture the empirical values (square markers) well for both confined diffusion and fBM. Moreover, the analytical covariance matrix without corrections (dashed curve) significantly deviates from the empirical values for the first and second covariance terms for confined diffusion and for fBM when $\alpha < 1$. These results demonstrate that the static and dynamic localization noise corrections are reliable for confined diffusion and fBM.

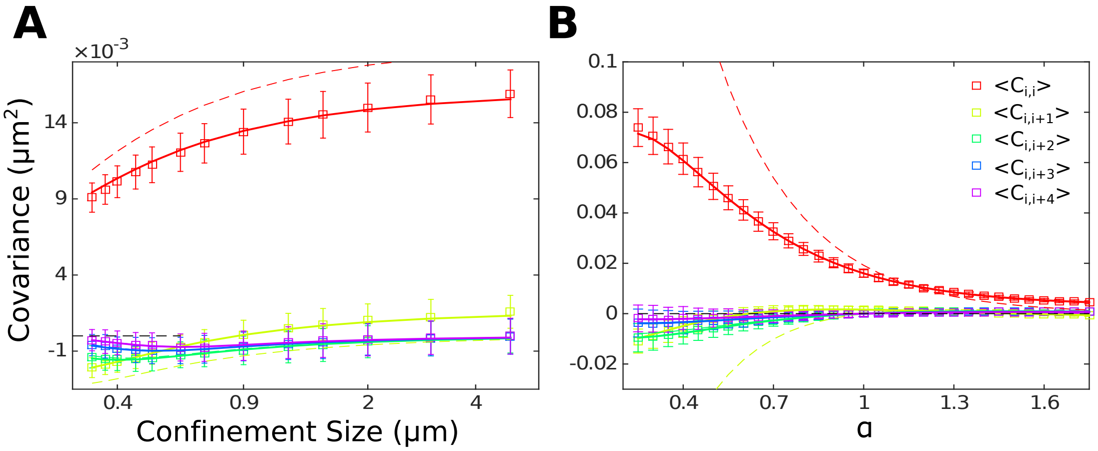


Figure S15. Comparison between theoretical and simulated values of the first five covariance matrix elements, for (A) confined diffusion and (B) fractional Brownian motion. Simulated covariance matrix elements, shown as the square markers, were calculated from 1,000 synthetic particle trajectories undergoing (A) confined diffusion for various confinement sizes and (B) fractional Brownian motion for various anomalous exponents with $D^{sim} = 0.3\ \mu\text{m}^2\text{s}^{-\alpha}$, $\sigma^{sim} = 0.04\ \mu\text{m}$, and $N$=100 steps. The error bars represent the standard error of the mean. The theoretical covariance matrix elements with localization noise are shown as the solid lines and without localization noise as the dashed lines.

[1] A. Einstein, *Investigations on the Theory of the Brownian Movement* (Courier Dover Publications, 1956).

[2] M. J. Saxton and K. Jacobson, Annual review of biophysics and biomolecular structure **26**, 373 (1997).

[3] H. Qian, M. P. Sheetz, and E. L. Elson, Biophysical journal **60**, 910 (1991).

[4] A. Kusumi, Y. Sako, and M. Yamamoto, Biophysical journal **65**, 2021 (1993).

[5] J.-H. Jeon and R. Metzler, Journal of Physics A: Mathematical and Theoretical **43**, 252001 (2010).

[6] J. D. Hamilton, *Time series analysis*, Vol. 2 (Princeton university press Princeton, 1994).

[7] A. S. Goldberger, *A course in econometrics* (Harvard University Press, 1991).

[8] N. Monnier, S.-M. Guo, M. Mori, J. He, P. Lénárt, and M. Bathe, Biophysical Journal **103**, 616 (2012).

[9] C. L. Vestergaard, P. C. Blainey, and H. Flyvbjerg, Physical Review E **89**, 022726 (2014).

[10] X. Michalet, Physical Review E **82**, 041914 (2010).

[11] G. Voisinne, A. Alexandrou, and J.-B. Masson, Biophysical journal **98**, 596 (2010).

[12] H. Qian, in *Processes with Long-Range Correlations* (Springer, 2003) pp. 22–33.

[13] B. B. Mandelbrot and J. W. Van Ness, SIAM review **10**, 422 (1968).

[14] K. I. Mortensen, L. S. Churchman, J. A. Spudich, and H. Flyvbjerg, nature methods **7**, 377 (2010).

[15] T. Savin and P. S. Doyle, Biophysical journal **88**, 623 (2005).

[16] A. J. Berglund, Physical Review E **82**, 011917 (2010).

[17] D. Montiel, H. Cang, and H. Yang, The Journal of Physical Chemistry B **110**, 19763 (2006).

[18] M. P. Backlund and W. Moerner, in *SPIE BiOS* (International Society for Optics and Photonics, 2015) pp. 933106–933106.
